# Supplementary material for: Analysis of Triplet Motifs in Biological Signed Oriented Graphs Suggests a Relationship Between Fine Topology and Function
Source: arXiv:1803.06520 source file (2019-07-10)
Supplement: Supplementary file 1 [file supplementary_1.pdf]

# Supplementary 1 – Triplets Counter Application

The application used for this analysis is distributed as a free java file (.jar) that can be run from command line or installed as a Cytoscape application.  It counts triplets, Closed and Linear, and it returns analysis results for further investigations. The Cytoscape App also plots Significance Profiles of the analyzed network.

## Command line application

```
Example:
java -jar TripletsCounter.jar \
             -s 0 -t 1 -e 2 -eal activation -eil inhibition \
             -d ";" -x 100 -i SIGNOR.csv -o Results

Where

 -d,--delimiter <arg>                     A character to split input text file
 -e,--edge <arg>                          Edge column index
 -eal,--edge_activation_label <arg>       Substring to identify activations (case insensitive)
 -eil,--edge_inhibition_label <arg>       Substring to identify inhibitions (case insensitive)
 -i,--input_file <arg>                    Input plain text file
 -o,--output_file_prefix <arg>            Output plain text files prefix
 -s,--source <arg>                        Source node column index
 -t,--target <arg>                        Target node column index
 -x,--random_iterations <arg>             Number of random graphs to generate for mean and
                                          st. Deviation calculation
```

This will produce two output files:

1) *prefix_summery.csv* with means and standard deviations for all motifs found in the analyzed network and the average occurrence in randomly generated networks with the same nodes, edges and activation/inhibition ratio. (Prefix is specified through the –o switch)
2) *prefix_list.csv* with the list of all nodes followed by all the motifs they are involved in. This second file can easily be used for statistical analysis and machine learning approaches. (Prefix is specified through the –o switch)

## Cytoscape App

The provided .jar file can be installed as a Cytoscape application. The user has to create a “Network View” and start the App from the dedicated Cytoscape menu option.

A pop-up configuration window asks the user to specify the edge attribute used to discriminate the two interaction signs (classes) to analyze (Activation/Inhibition). Other than this, the application can

randomly generate networks similar to the one defined by the user and calculate motifs z-scores and significance profiles.

When the analysis is completed the Cytoscape App shows a floating window which reports results already partially analyzed.

The floating window contains 5 main tabs.

1) *Closed Triplets* which reports the relative abundance of each closed triangle in the network.
2) *Linear Triplets* which reports the relative abundance of linear triplets in the network.
3) *Significance Profile* reports the profile of the network analyzed as a line chart.
4) *Data* reports for each motif its abundance in the analyzed network and in randomly generated ones together with standard deviation, z-scores and significance profile score.
5) *Motifs Table* contains the entire list of motifs for each node in the network for further analysis and possibly machine learning classification approaches.

The following figure schematically illustrates the steps to take to analyze a toy network.

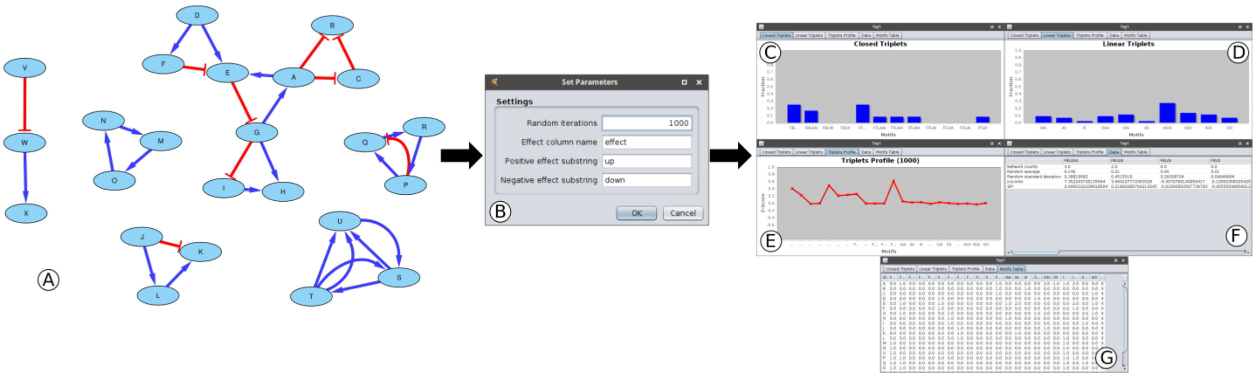


Figure 1. Cytoscape App to count Triplets. The analysis stars with a network to analyze, A) shows a toy network. Next, the user specifies analysis parameters B) then, after clicking OK the App calculates random network, if needed, and reports results. C) and D) are the relative abundance of each counted motif. E) is the significance profile. F) Reports statistics against randomly generated networks. G) Lists all nodes and motifs in the network. Each chart and table is exportable through the right click mouse menu.
